# Supplementary material for: Nonlinear dispersion in wave-current interactions
Source: arXiv:2108.05213 source file (2021-08-11)
Supplement: Supplementary file 1 [file Appendix.tex]

\appendix

%%%%%%%%%%%%%%%%%%%%%%%%%%%%%%%%%%%%%%%%%%%%%%%%%%%
